# Supplementary material for: ZodiAq: An Isotropic Flagella-Inspired Soft Underwater Drone for Safe Marine Exploration
Source: arXiv:2503.19556 source file (2025-03-25)
Supplement: Supplementary file 1 [file SupplementaryMaterial.pdf]

# Supplementary Materials for ZodiAq: An Isotropic Flagella-Inspired Soft Underwater Drone for Safe Marine Exploration

Anup Teejo Mathew et al.

Corresponding author: anup.mathew@ku.ac.ae

February 21, 2024

## 1 Details of Design, Fabrication, and Assembly

The development of a soft robot prototype, such as ZodiAq, encompasses several critical stages including the mechanical design, selection of components, fabrication of parts, design, and execution of electrical connections, and assembly. While the summary of the design and fabrication process of the prototype is provided in the manuscript, this section provides details of the process.

### 1.1 Design and Fabrication of Components

The shell frame of the prototype is constructed from a 9mm thick Polyvinyl Chloride (PVC) sheet. Individual faces of the dodecahedron are machined using a CNC (Computerised Numerical Control) machine and chemically bonded with PVC glue. Two 3D-printed racks are mounted inside the frame to assemble internal components. For the shell's faces, transparent pentagonal sheets made from a 5mm thick polycarbonate are fabricated. Motor canister assemblies are constructed by integrating DC motors, shaft couplers, PVC canisters, and O-rings. We used high torque (0.88 Nm) and low RPM (130 RPM) DC motors. The motor canister assemblies are first adhered to the transparent plates using epoxy glue, followed by a coating of silicone glue. These plates are then fastened to each face of the shell frame, using an O-ring and ten M3 screws to ensure waterproofing. Flagella are manufactured by a molding process using Mold Star™ 30 silicone rubber. A 3D-printed part is inserted into the mold to make the hook area rigid and enable mounting of the flagellum into the motor shaft. Figure 1 explains the fabrication process of these components.

ZodiAq uses a Raspberry Pi 4 Model B as its central unit. The actuators are controlled by the Raspberry Pi through DC motor drivers: Adafruit DC Motor HAT (Hardware Attached on Top), which can control the velocity of four motors in both clockwise and counterclockwise directions using Pulse width modulation (PWM)

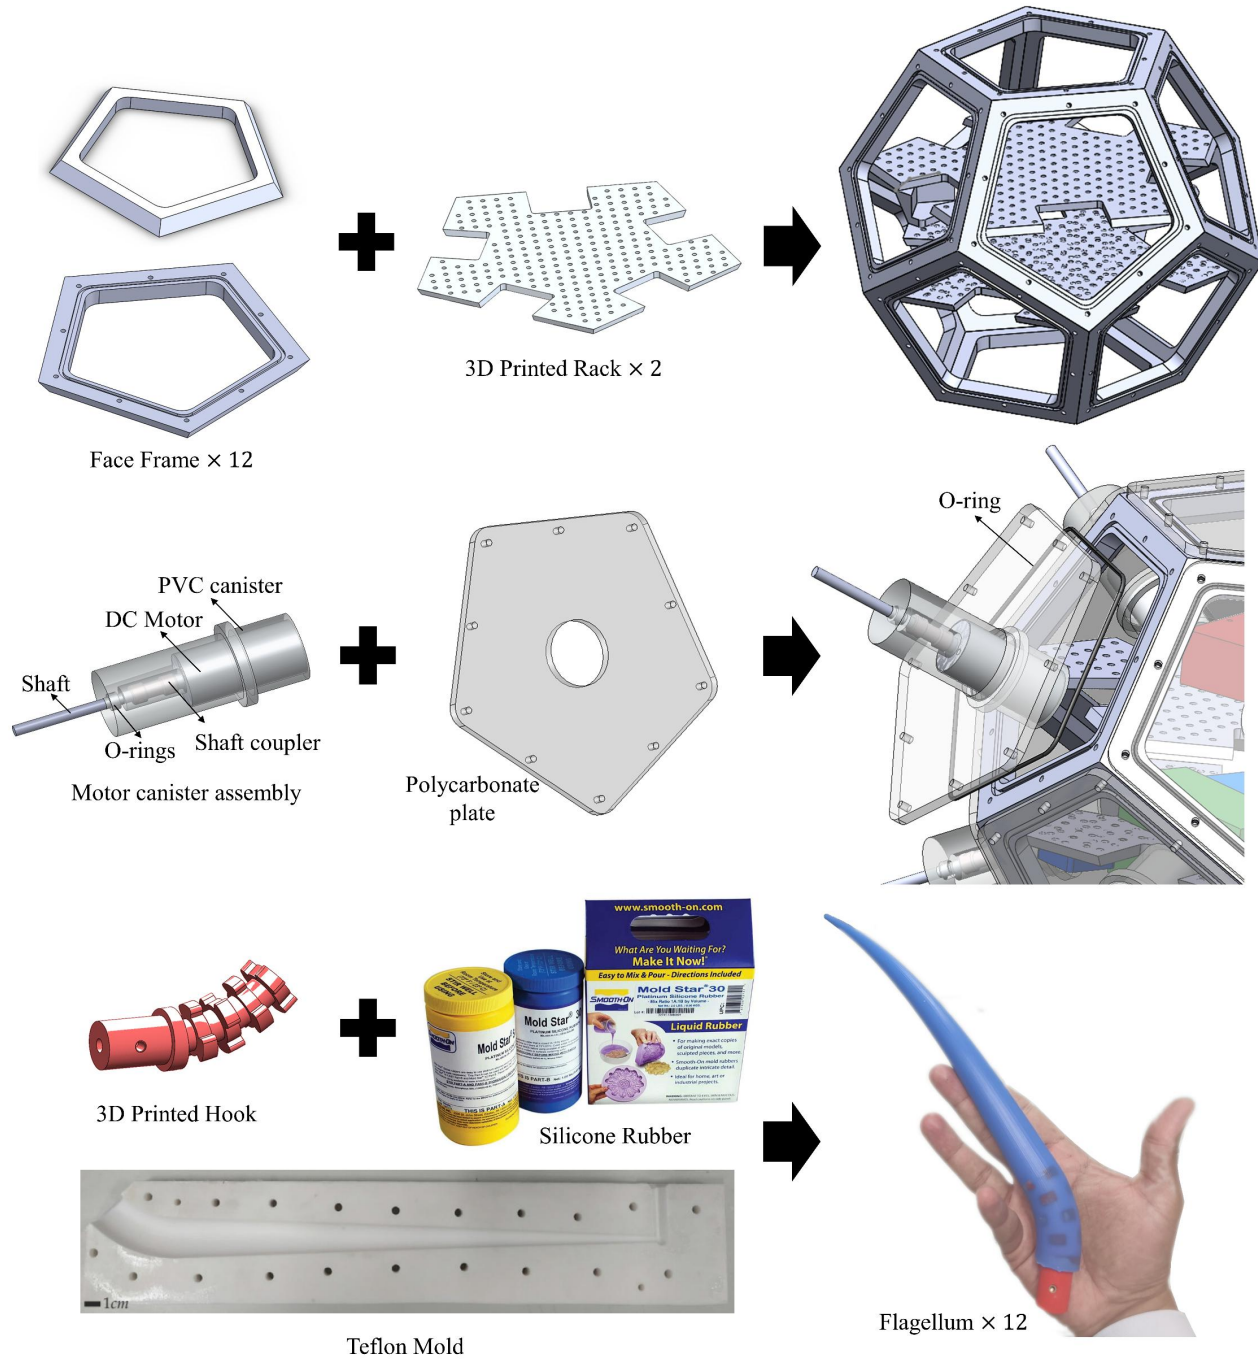

Figure 1: Fabrication of the frame of the dodecahedral shell, motor canister assembly with transparent face plates, and flagellum

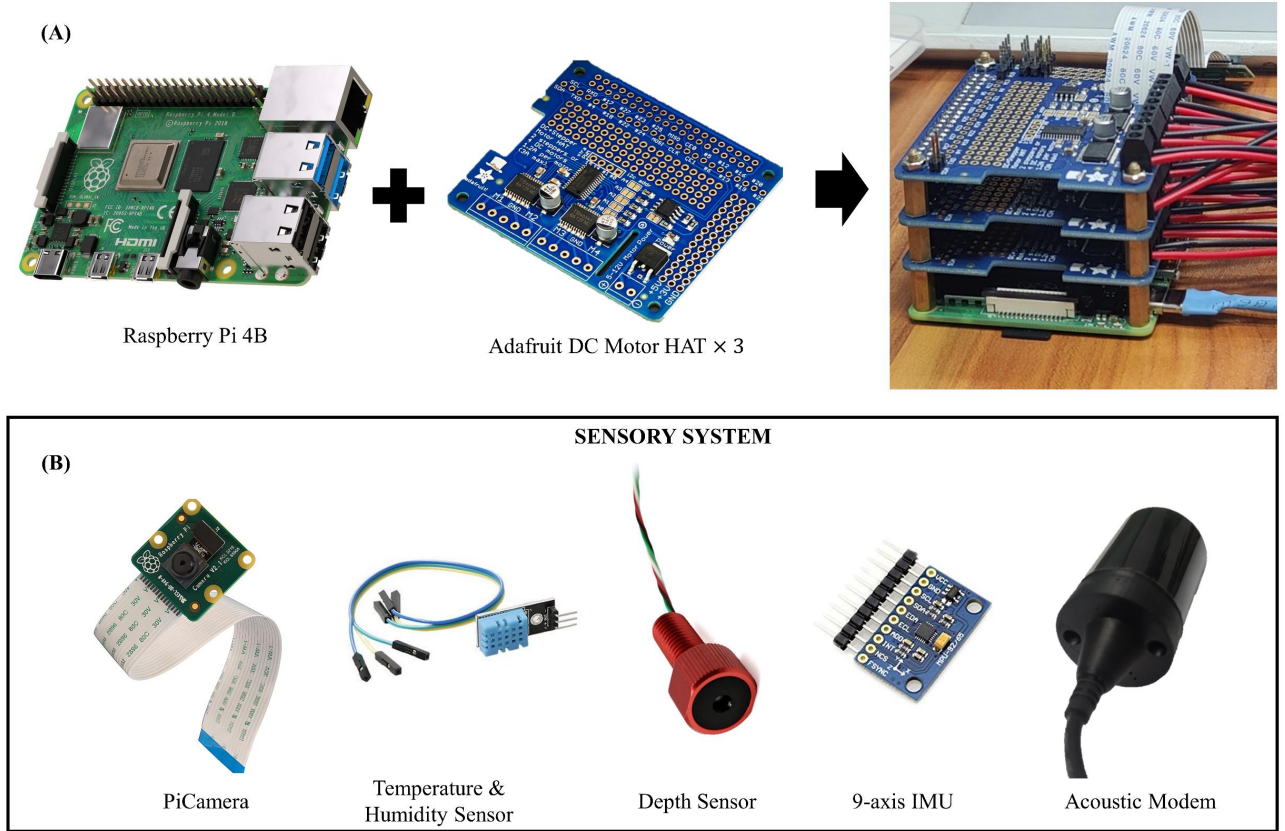

Figure 2: Raspberry Pi and Accessories: (A) Assembly of Raspberry Pi with HATs. (B) Sensory system of ZodiAq

signals. Therefore, to accommodate all 12 motors, three HATs are stacked on the Raspberry Pi (Figure 2A). The sensory system of ZodiAq consists of the following parts. It utilizes the PiCamera, the default camera of the Raspberry Pi, for video capture. The camera is arranged inside, facing outward through one of the transparent faces. For internal monitoring, a temperature and humidity sensor (DHT11) is used to detect any overloading or water leakages. Depth feedback is provided by a depth sensor (MS5837-30BA), and for motion and orientation sensing, a 9-axis Inertial Measurement Unit (MPU-9250) is used. The depth sensor is mounted on the bottom face, while both the IMU and the temperature-humidity sensor are assembled on the top rack. ZodiAq employs an acoustic modem (Succorfish Nanomodem v3) for communication. The modem is attached to the top face using epoxy glue. All these components are connected to the central Raspberry Pi unit, forming the core of ZodiAq's sensory system (Figure 2B).

## 1.2 Electrical Connections and System Integration

The schematic of the electrical connection of various components of ZodiAq is shown in Figure 1B of the manuscript. The Raspberry Pi and the motors are powered by six 7.4V 2S Lithium Polymer (LiPo) batteries. They are split into two sets, each comprising three batteries connected in parallel. One set powers the Raspberry Pi, while the other operates the HATs which control the motors. Each LiPo battery is connected to a Battery Management System (BMS) for the uniform charging of individual cells. There are two external charging ports available, allowing for the individual charging of each battery set. To prevent short circuits due to the charging

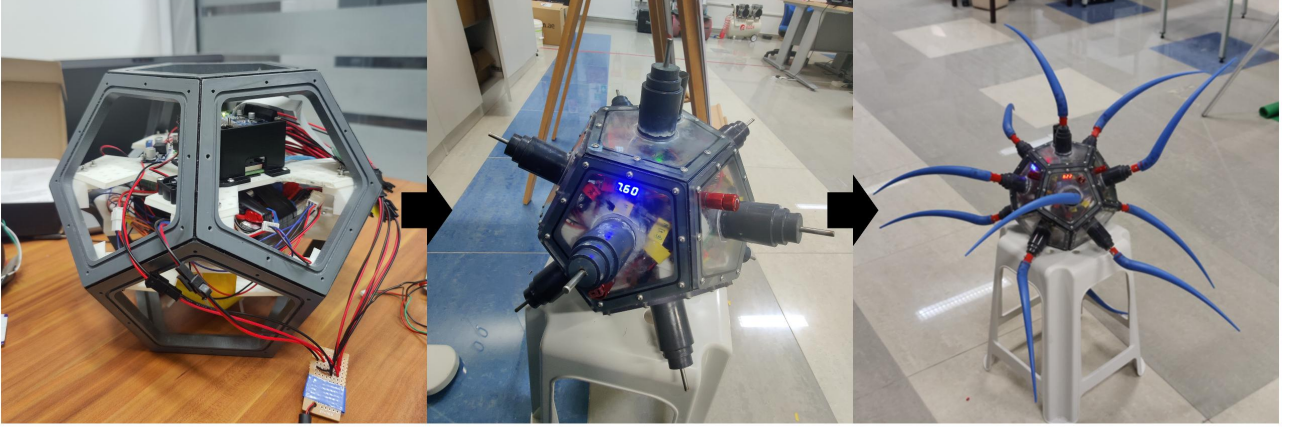

Figure 3: Assembly of ZodiAq

ports being exposed to water, a charging circuit has been designed using a 9V electromagnetic relay switch.

Similarly, the operating circuit is activated using an external waterproof rotary switch. The first set of batteries powers a buck converter, which steps down the voltage from 7.4V to 5V. The output of this converter is then used to power the Raspberry Pi as well as the two internal DC fans, which ensure adequate heat circulation within the shell. ZodiAq's sensory system is connected to the Raspberry Pi via its Camera Serial Interface (PiCamera), digital pins (Temperature-Humidity sensor, depth sensor), I2C interface (IMU), and USB ports (acoustic modem). Meanwhile, the second set of batteries is responsible for powering all three HATs, each connected to four motors: HAT1 to the first four motors, HAT2 to the next four, and HAT3 to the last four. The motor driver, receiving velocity commands from the Raspberry Pi ranging from -1 to 1, generates PWM signals to control motor rotation. Positive and negative command values correspond to clockwise (CW) and counterclockwise (CCW) rotations, respectively, enabling precise speed and directional control.

All internal components are assembled across two racks: batteries on the lower rack and the Raspberry Pi, along with its accessories on the upper rack. A ballast of approximately 4 kg is attached to the lower rack. This strategic placement lowers the center of mass below the center of buoyancy, the geometric center, thereby achieving neutral and stable buoyancy for the prototype. Based on geometric assumptions, we estimate a vertical shift of 3.5 cm. Figure 3 shows the assembly process of the prototype, including the assembly of internal components, faces, and flagella.

## 2 Mathematical Modeling

### 2.1 Summary of GVS Model

The GVS model parameterizes the distributed strain field of the Cosserat rod and the joint twists of the rigid joints using basis functions ( $\Phi_{\xi_i}$ ):

$$\xi_i = \Phi_{\xi_i} q_i \quad \text{for rigid joints} \quad (1a)$$

$$\xi_i(X_i) = \Phi_{\xi_i}(X_i) q_i + \xi_i^*(X_i) \quad \text{for soft bodies,} \quad (1b)$$

where  $\xi_i$  is the distributed strain field of the  $i^{th}$  soft body or the joint twist of the  $i^{th}$  rigid link,  $q_i$  is the generalized coordinates of the soft body or rigid joint,  $\xi_i^*$  is the reference strain field, and  $X_i \in [0, 1]$  is the normalized curvilinear abscissa along the centerline of the soft body.

ZodiAq is a branched hybrid system with soft and rigid parts. It consists of a central rigid shell, which is free to translate and rotate in all directions. Protruding from the shell are 12 motor shafts, each modeled as a 1 DoF revolute joint rotating about its local x-axis. The flagella, rigidly connected to each shaft, is composed of two parts: the hook, a rigid body with a  $45^\circ$  pre-curvature, and the soft flagellum. Hence, for the free joint of the shell,  $\Phi_{\xi_i} = \mathbf{I}(6)$ , for the revolute joints of the shafts,  $\Phi_{\xi_i} = [1 \ 0 \ 0 \ 0 \ 0 \ 0]^T$ , and for the soft body  $\Phi_{\xi_i}(X_i) \in \mathbb{R}^{6 \times n_i}$  is a function of  $X_i$ . We model the flagella as an inextensible Kirchhoff rod, a subclass of the Cosserat rod, incorporating torsion and bending. We impose a linear ( $1^{st}$  order) strain parameterization, resulting in six degrees of freedom (6 DoFs) per flagellum. The basis function is given by:

$$\Phi_{\xi_i}(X_i) = \begin{bmatrix} 1 & 2X_i - 1 & 0 & 0 & 0 & 0 \\ 0 & 0 & 1 & 2X_i - 1 & 0 & 0 \\ 0 & 0 & 0 & 0 & 1 & 2X_i - 1 \\ 0 & 0 & 0 & 0 & 0 & 0 \\ 0 & 0 & 0 & 0 & 0 & 0 \\ 0 & 0 & 0 & 0 & 0 & 0 \end{bmatrix} \quad (2)$$

The GVS model employs the exponential map of Lie Algebra to compute the forward and differential kinematics of the system, mapping  $q$  and  $\dot{q} \rightarrow g_i(X_i)$ ,  $J_i(X_i)$ , and  $\dot{J}_i(X_i)$ , where  $q \in \mathbb{R}^n$  ( $n = \sum n_i$ ) is the vector of generalized coordinates of the system, encompassing  $q_i$  of rigid joints and soft bodies,  $g_i \in SE(3)$  is the configuration of  $i^{th}$  body with respect to the spatial frame, and  $J_i \in \mathbb{R}^{6 \times n}$  is the geometric Jacobian. Projecting the system's free dynamics with the geometric Jacobian through D'Alembert's principle enables the formulation of the generalized dynamic equation of motion in the standard Lagrangian form:

$$M(q)\ddot{q} + (C(q, \dot{q}) + D(q))\dot{q} + Kq = B(q)u + F(q, \dot{q}), \quad (3)$$

where  $M(q)$ , is the generalized mass matrix,  $C(q, \dot{q})$  is the generalized Coriolis matrix,  $D(q)$  is the generalized elastic damping matrix,  $K$  is the generalized stiffness matrix,  $B(q)$  is the generalized actuation matrix,  $F(q, \dot{q})$  is the vector of generalized external forces, and  $u$  is the vector of applied motor torques.

## 2.2 Fluid Interaction Forces

The robot experiences external force due to gravity, buoyancy, added mass, drag, and lift forces [1]. For rigid links, external forces are modeled as point wrenches ( $\mathcal{F}$ ) acting at the geometric center, while for soft links, they are treated as distributed loads ( $\bar{\mathcal{F}}$ ). The subscript  $i$  has been intentionally omitted for simplicity. We

have,

$$\mathcal{F} = \mathcal{F}_G + \mathcal{F}_B + \mathcal{F}_D + \mathcal{F}_A \quad (4a)$$

$$\bar{\mathcal{F}} = \bar{\mathcal{F}}_G + \bar{\mathcal{F}}_B + \bar{\mathcal{F}}_D + \bar{\mathcal{F}}_A \quad (4b)$$

The combination of gravity and buoyancy force is given by:

$$\mathcal{F}_G + \mathcal{F}_B = (\mathcal{M} - \rho_w V_{ext} \mathbf{I}_6) \mathcal{G} \quad (5a)$$

$$\bar{\mathcal{F}}_G + \bar{\mathcal{F}}_B = (1 - \rho_w / \rho) \bar{\mathcal{M}} \mathcal{G}, \quad (5b)$$

where,  $\mathcal{M}$  is the inertia matrix of a rigid body,  $\bar{\mathcal{M}}$  is the linear inertia density of the cross-section of the soft body,  $\rho$  is the density of the body,  $\rho_w$  is the density of water, and  $\mathcal{G}$  is the gravitational acceleration twist expressed in the local frame.

As a body moves underwater, it experiences drag and lift forces due to the interaction with the surrounding fluid. The model of drag and lift force on the bodies are given by:

$$\mathcal{F}_D = -\mathcal{D} \|\boldsymbol{\nu}\| \boldsymbol{\eta} \quad (6a)$$

$$\bar{\mathcal{F}}_D(X) = -\bar{\mathcal{D}}(X) \|\boldsymbol{\nu}(X)\| \boldsymbol{\eta}(X), \quad (6b)$$

where,  $\boldsymbol{\nu}$  is the translational part of the velocity twist  $\boldsymbol{\eta}$  while,  $\mathcal{D}$  and  $\bar{\mathcal{D}}$  are the screw matrices of drag and lift coefficients. The form of drag-lift matrix of the shell  $\mathcal{D}_{shell}$ , shaft  $\mathcal{D}_{shaft}$ , hook  $\bar{\mathcal{D}}_h$ , and flagellum  $\bar{\mathcal{D}}_f$  are given by:

$$\mathcal{D}_{shell} = \frac{1}{2} \rho_w \cdot \text{diag}[C_x A_x R_s^3, C_y A_y R_s^3, C_z A_z R_s^3, C_x A_x, C_y A_y, C_z A_z] \quad (7a)$$

$$\mathcal{D}_{shaft} = \frac{1}{2} \rho_w \cdot \text{diag}[0, 0, 0, C_x A_x, C_y A_y, C_z A_z] \quad (7b)$$

$$\bar{\mathcal{D}}_{h,f}(X) = r_{h,f}(X) \rho_w \begin{pmatrix} \mathbf{0}^{4 \times 4} & \mathbf{0}^{4 \times 2} \\ \mathbf{0}^{2 \times 4} & \begin{matrix} C_D & -C_L \\ C_L & C_D \end{matrix} \end{pmatrix} \quad (7c)$$

where  $R_s$  Shell's equivalent radius when approximated as a sphere,  $A_x$ ,  $A_y$ , and  $A_z$  are the cross-sectional areas of the body in the x-, y-, and z-axes directions,  $r$  is the radius of the cross-section, and  $C_{(\cdot)}$  are empirical values of lift and drag coefficients estimated experimentally [1].

Added mass ( $\mathcal{M}_A$ ) is an effect that arises when a body moves through a fluid, resulting from the fluid's inertia opposing the body's motion. The action of added mass is given by:

$$\mathcal{F}_A = -\mathcal{M}_A \dot{\boldsymbol{\eta}}, \quad \bar{\mathcal{F}}_A = -\bar{\mathcal{M}}_A \dot{\boldsymbol{\eta}}, \quad (8)$$

where  $\dot{\boldsymbol{\eta}}$  is the screw acceleration twist. We compute the added mass on the shell of ZodiAq by assuming it to be a sphere submerged in infinite fluid. The simplified added mass of the shell  $\mathcal{M}_{Ashell}$ , shaft  $\mathcal{M}_{Ashaft}$ , hook  $\overline{\mathcal{M}}_{Ah}$ , and flagellum  $\overline{\mathcal{M}}_{Af}$  are given by:

$$\mathcal{M}_{Ashell} = \rho_w V_{shell} \cdot \text{diag}[0, 0, 0, 0.5, 0.5, 0.5] \quad (9a)$$

$$\mathcal{M}_{Ashaft} = \rho_w V_{shaft} \cdot \text{diag}[0, 0, 0, 0, B_y, B_z] \quad (9b)$$

$$\overline{\mathcal{M}}_{Ah,f}(X) = \rho_w \pi r_{h,f}^2(X) \cdot \text{diag}[0, 0, 0, 0, B_y, B_z], \quad (9c)$$

where  $B_y$  and  $B_z$  are the added mass coefficients in the y and z axes. Since the force is linear with respect to  $\dot{\boldsymbol{\eta}}$  (according to equation (2.2)), it essentially acts as adding a virtual mass to the body's mass. Hence, the generalized mass ( $\boldsymbol{M}$ ) and Coriolis ( $\boldsymbol{C}$ ) matrix are computed by incorporating the added mass of individual bodies. Meanwhile, all other external force components are projected into the generalized force vector  $\boldsymbol{F}$ .

After evaluating the terms in the equation (3), it is integrated in time using an ODE integrator to solve for  $\boldsymbol{q}(t)$  and  $\dot{\boldsymbol{q}}(t)$ .

### 3 Creating ZodiAq's Digital Twin

SoRoSim (Soft Robot Simulator) is a Graphic User Interface (GUI) based MATLAB toolbox that can analyze open-, closed-, and branched hybrid robots under various external load and actuation scenarios [2]. We used the toolbox to create a digital twin of ZodiAq. This section documents the creation of the digital twin of the robot.

#### 3.1 Defining Links and the Linkage

SoRoSim uses MATLAB class objects to model links (`SorosimLink`) and combine them to form linkages (`SorosimLinkage`). Links are the building blocks of any system modeled in SoRoSim and are categorized into two types: Soft and Rigid. The ZodiAq is a hybrid, branched linkage with 37 links that are classified into four `SorosimLink` class objects: Shell, Shaft, Hook and Flagellum. These links are created in SoRoSim by entering the appropriate material and geometric properties when prompted by the GUI. Table 1 outlines the geometric and material properties of each link.

Once these `SorosimLinks` are created, we combine them to create the linkage of ZodiAq. The reference frame of the Shell, located at its geometric center (GC), is aligned with the global frame. Since the joint of the shell was defined as a free joint during link creation, a corresponding basis function, as described in Section 2.1, is automatically assigned to it. After this, we incorporated the second link, the Shaft. We used a transformation matrix  $\boldsymbol{g}_f$  to accurately position and orient the Shaft relative to the Shell's reference frame. The value of  $\boldsymbol{g}_f$  depends on the face of the dodecahedron to which the shaft is assembled. After the assembly, we define the Shaft's basis function by specifying that the revolute joint rotates about the local x-axis of the Shaft's frame

Table 1: Geometric and material properties of links

| Property                    | Shell* | Shaft    | Hook   | Flagellum          |
|-----------------------------|--------|----------|--------|--------------------|
| Link type                   | rigid  | rigid    | soft   | soft               |
| Base joint type             | Free   | Revolute | Fixed  | Fixed              |
| Radius ( $m$ )              | -      | 0.002    | 0.0125 | $0.0125 - 0.29X_i$ |
| Length ( $m$ )              | -      | 0.020    | 0.050  | 0.300              |
| Density ( $kg/m^3$ )        | -      | 7960     | 1062   | 1062               |
| Elastic Modulus ( $N/m^2$ ) | -      | -        | -      | 666190             |
| Pisson's ratio              | -      | -        | -      | 0.5                |
| Material Damping ( $Pa.s$ ) | -      | -        | -      | 11200              |

\* Geometric and material properties of the shell are modified by a custom function.

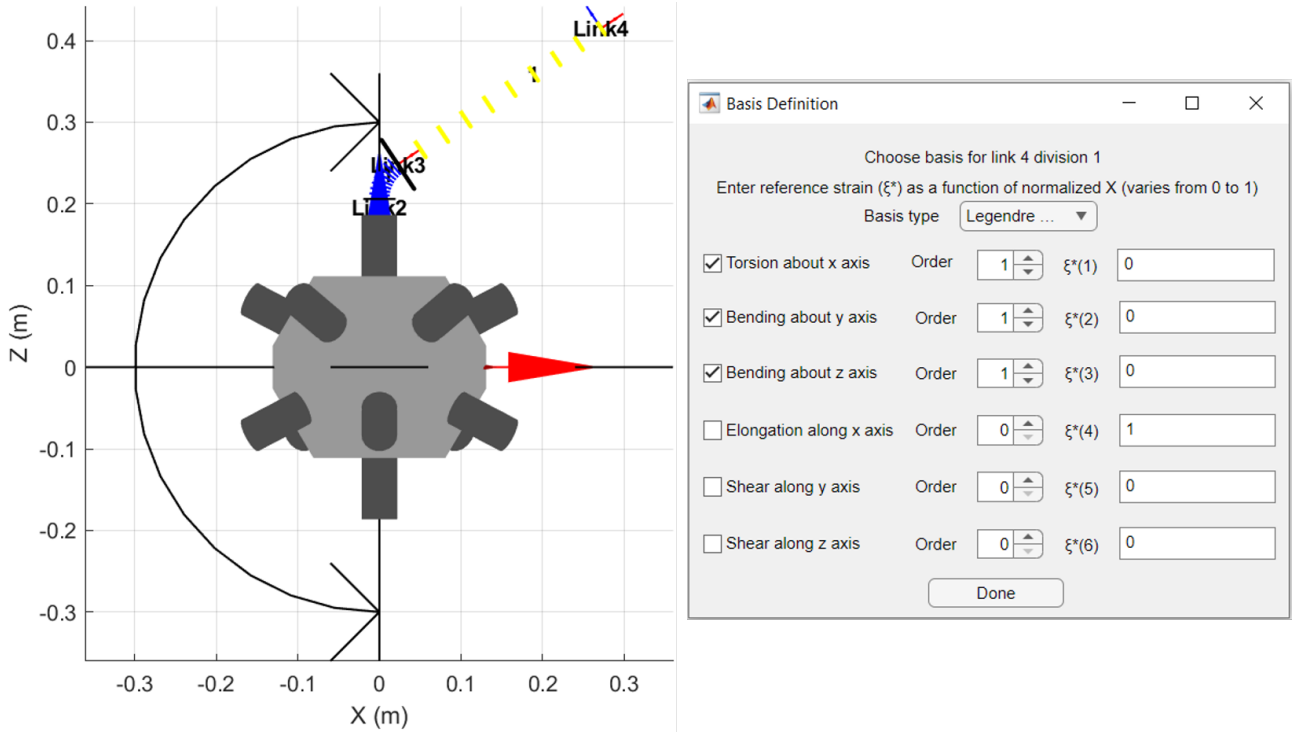

Figure 4: GUI showing the process of specifying the active modes of deformation and their order for a soft link

(Section 2.1). Following this, we assembled the Hook at the tip of the shaft. For the Hook we define a reference strain,  $\xi_i^* = [0 \ \pi/(4l_h) \ 0 \ 1 \ 0 \ 0]^T$ , where  $l_h$  is the length of the Hook. By assigning it with 0 DoF, we effectively model it as a curved rigid link. Finally, a flagellum is assembled at the tip of the Hook. The active modes of deformation of the Flagellum and their order are specified with the help of the GUI as shown in Figure 4. We activated torsion about the x-axis, along with bending about both the y-axis and the z-axis, with linear strain parameterization (1st order). This completes the assembly of the first branch. The same process is repeated 11 more times to assemble actuators on each face of the shell.

After completing the assembly, external forces and actuators are specified. Gravity is defined to be in the negative z-axis using the GUI. The revolute joints of all shafts are designated as actuators, controlled by joint angles. Following these specifications, the digital twin of ZodiAq is established as a **SorosimLinkage**. The change in mechanical properties due to the non-trivial shape of the Shell, the forces due to fluid interaction, and the control law are integrated into the system using separate MATLAB functions described in the next section.

### 3.2 Custom Properties, External Forces, and Actuation

Due to the arrangement of internal components, the GC and Centre of Mass (CM) of the Shell are not coincident, and the inertia matrix is not a diagonal matrix [1]. For ZodiAq, we estimated a vertical shift of  $d_{CM} = 3.5\text{cm}$  between the GC and the CM. Based on the geometry of the dodecahedron and the motor canister assembly, the volume of the shell is calculated. Assuming neutral buoyancy, the mass is computed as  $m = \rho_w V_{ext} = 8.57\text{kg}$ . The moment of inertia of the dodecahedral shell about each axis is computed as follows:

$$I_x = I_y = \frac{ms^3(39\phi + 28)}{150} + md_{CM}^2, \quad I_z = \frac{ms^3(39\phi + 28)}{150}, \quad (10)$$

where  $s = 0.1\text{m}$  is the edge length of the dodecahedron,  $\phi$  is a constant equal to  $\frac{1+\sqrt{5}}{2}$ , and the term  $md_{CM}^2$  comes from the parallel axis theorem to account for the vertical displacement of the CM. As the shift is along the z-axis,  $I_z$  remains unchanged. The updated inertia matrix  $\mathcal{M}_{shell}$  of the shell is given by:

$$\mathcal{M} = \begin{pmatrix} \mathcal{I} & m\tilde{\mathbf{c}} \\ -m\tilde{\mathbf{c}} & m\mathbf{I}_3 \end{pmatrix}, \quad (11)$$

where,  $\mathcal{I} = \text{diag}[I_x, I_y, I_z]$ ,  $\mathbf{c} = [0, 0, d_{CM}]^T$ , and  $\tilde{\mathbf{c}}$  denotes the skew-symmetric matrix form of the vector  $\mathbf{c}$ . A MATLAB file called `MoI_update.m` computes and updates the inertia matrix of the Shell.

SoRoSim employs a custom MATLAB script, `CustomExtForce.m`, allowing users to model various types of external forces. The toolbox accesses this file during the dynamic simulation if the `CEFP` (Custom External Force Present) property of the `SorosimLinkage` is enabled. We implement the models (Section 2.2) of buoyancy and drag-lift forces in this file (note that gravity is a default external force that can be enabled during linkage creation). We computed the drag-lift matrices (7) using a function called `DragLiftMatrix.m`, and saved the values as a custom property (CP1) of the `SorosimLinkage`. For the shell, we assume a spherical shell with a radius  $R_s = 0.11\text{m}$  to simplify the calculations. By the same assumption, we have  $A_x = A_y = A_z = \pi R_s^2$ . The drag-lift coefficients used are as follows:  $C_x = C_y = C_z = 2.5$  for the shell;  $C_x = 0.01$ ,  $C_y = C_z = 2.5$  for the shaft;  $C_D = 1.1$ ,  $C_L = -0.1$  for the hook; and  $C_D = 1.1$ ,  $C_L = -0.3$  for the filament. Similarly, the added mass (9) of each body is pre-computed using the file `AddedMass.m`, and the values are saved in the property called `M_added` of the `SorosimLinkage`. The added mass coefficients of the shaft are  $B_y = B_z = 1.5$ , while for the hook and flagellum, they are set to  $B_y = B_z = 0.6$ . As previously discussed, `M_added` is used for calculating the matrices  $\mathbf{M}$  and  $\mathbf{C}$  of equation (3).

The revolute joints of the shafts are actuated by joint angles, allowing users to specify actuation inputs as functions of time. The dynamic simulation is initiated by entering `ZodiAq.dynamics` in MATLAB's command window. Following this, the user can input joint angles as prompted by the GUI. Figure 2C in the manuscript illustrates the results of a dynamic simulation using an angle input of `2*pi*t` (60 RPM) for motors M6, M8, M9, and M11, while setting 0 for the remaining motors. Another method for specifying actuation involves utilizing the `CustomActuatorStrength.m` file. Initially, one must enable the `CAS` (Custom Actuation Strength) property

of the `SorosimLinkage` by entering `ZodiAq.CAS=true` in the MATLAB command window. Subsequently, the file can be modified to define the actuation inputs. We used this file to implement a control law for ZodiAq's navigation. The implemented control law is described in the next section. Interested readers can simulate the digital twin in MATLAB using the SoRoSim files available at the GitHub link provided in [3].

## 4 Control Design for Robot Navigation

In this section, we present a simplified model to develop the motion control of the robot for performing navigation. This model is essentially obtained by representing the system as a solid body evolving in 3D and subject to the forces and moments generated by the rotation of the motors at the centre of each face (see Figure 6).

### 4.1 Simplified Dynamic Model

The simplified dynamic model used for the development of the control law is derived under the following assumptions:

- The main structure of the robot is supposed to be rigid.
- The structure is supposed to be symmetrical respect to its vertical axis.
- The system mainly rotates only around its vertical axis due to its inherent stability by design (CM is below the center of buoyancy), permitting significant rotations solely around this axis. As a result, small angle approximations have been employed for the other two angles.
- We assume perfect neutral buoyancy of the system, the effect of the gravity and buoyancy can be neglected.
- The flagellum rotation generates a thrust and an angular moment which are proportional to the flagellum's speed and they are perpendicular to its face.
- All flagella are equal, meaning that each of these appendages shares identical properties, such as length, material composition, and structural characteristics.

As the motor rotates, the soft flagella interact with the surrounding fluid and deform, resembling an helical shape that depends of many parameters, including the stiffness of the material and the rotational speed of the motor. This interaction generates forces and torques exerted during the rotation of the flagella. In total, three torques ( $m_x$ ,  $m_y$  and  $m_z$ ) and three forces ( $f_x$ ,  $f_y$  and  $f_z$ ) are produced. The results presented in [1] showed that only two reaction forces are not null, on average, during the rotation of a single flagellum: the propulsive thrust  $f_x$  and the out-of-plane torque  $m_x$ . We simulated the rotation of the flagellum at different angular velocities using our toolbox SoroSim to obtain the reaction forces and moments at the base generated by the rotation. The angular velocity range  $[0 - 4]\pi$  rad/s was chosen to align with the operational capabilities of the selected motors inside the water. Figure 5A and Figure 5B show the reaction forces for a rotation speed of  $\pi$  rad/s. We observe that only the propulsive thrust  $f_x$  and the out-of-plane torque  $m_x$  are not null during

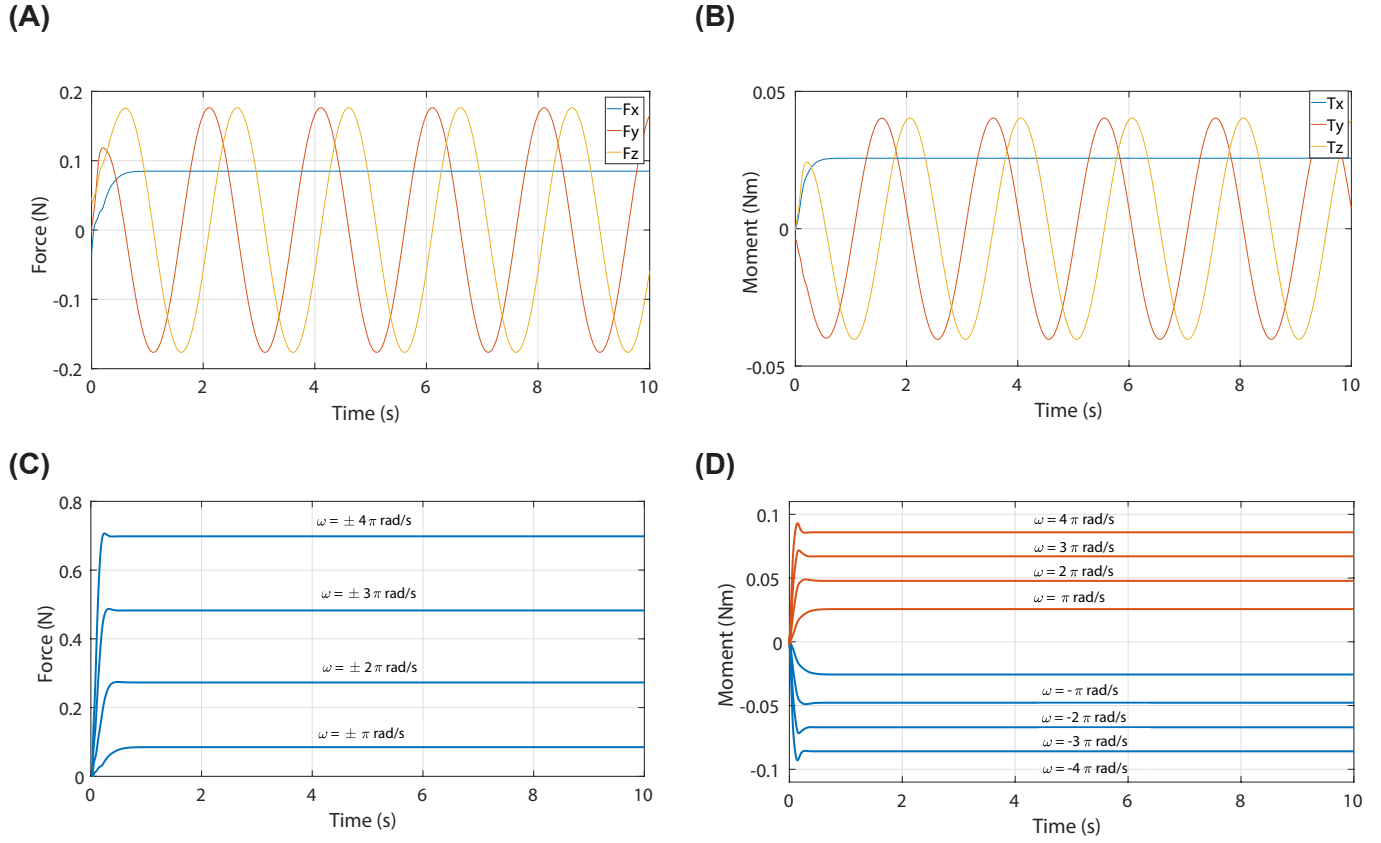

Figure 5: Constraint torques and forces exerted at the base of the flagella, obtained from the theoretical simulations at different speeds. It can be noticed that only the propulsive thrust  $f_x$  and the out-of-plane torque  $m_x$  have a nonzero mean.

the rotation, matching the results obtained in [1]. Figure 5C and Figure 5D represent  $f_x$  and  $m_x$  for different angular velocities. Considering the steady state values of the functions and the range of actuation of the motors, the reaction forces are approximated as first-order functions of the angular speed. Specifically, propulsive thrust is approximated as  $f_x = a_1 \cdot |\omega|$ , and the moment is approximated as  $m_x = a_2 \cdot \omega$  being  $a_1 = 0.065$  and  $a_2 = 0.0064$ .

The rotation of a rigid body in space can be parameterized using the well-known Euler angles. Then, the complete rotation matrix is the product of the three successive rotations  $\mathbf{R}(\phi, \theta, \psi) \in SO(3)$ . Assuming small angles in  $\phi$  and  $\theta$ , we have that  $\mathbf{R}(\phi, \theta, \psi) \approx \mathbf{R}(\psi)$ . The rotation dynamics is modelled using Euler-Lagrange Formalism.

$$\Gamma_i = \frac{d}{dt} \left( \frac{\delta L}{\delta \dot{q}_i} \right) - \frac{\delta L}{\delta q_i} \quad (12)$$

Let us consider earth fixed frame  $E$ , body fixed frame  $B$  and the frames of the faces  $C_i$  as seen in Figure 6A. In this simplified model, we position the origin of the body-fixed frame at the CM of the system. The airframe orientation in space is given by a rotation  $\mathbf{R}(\psi)$  from  $B$  to  $E$ . The mechanical symmetry of the system allows us to neglect the inertia products and consider a diagonal inertia matrix. The three equations that describe the dynamics of the rotations are:

$$\begin{bmatrix} I_x \ddot{\phi} \\ I_y \ddot{\theta} \\ I_z \ddot{\psi} \end{bmatrix} = \begin{bmatrix} \dot{\theta} \dot{\psi} (I_y - I_z) \\ \dot{\phi} \dot{\psi} (I_z - I_x) \\ \dot{\phi} \dot{\theta} (I_x - I_y) \end{bmatrix} + \begin{bmatrix} \tau_\phi \\ \tau_\theta \\ \tau_\psi \end{bmatrix} \quad (13)$$

The detailed mathematical derivation of (13) is provided in Appendix B.2 of [4]). Conversely, the dynamics of the translations are developed using Newton-Euler Formalism:

$$m \begin{bmatrix} \ddot{x} \\ \ddot{y} \\ \ddot{z} \end{bmatrix} = \mathbf{R}(\psi) \begin{bmatrix} f_x \\ f_y \\ f_z \end{bmatrix} \quad (14)$$

where  $x$ ,  $y$  and  $z$  are the position in the earth fixed frame E. Then, we can express equations (13) and (14) in the following matrixial form:

$$\mathbf{M} \ddot{\mathbf{q}} + \mathbf{C}(\mathbf{q}, \dot{\mathbf{q}}) \dot{\mathbf{q}} = \mathbf{u} \quad (15)$$

where

$$\boldsymbol{\Upsilon} = \begin{bmatrix} \mathbf{I}_{3 \times 3} & \mathbf{0}_{3 \times 3} \\ \mathbf{0}_{3 \times 3} & \mathbf{R} \end{bmatrix}$$

and  $\mathbf{q} = [\phi, \theta, \psi, x, y, z]^T$  is the vector of generalized coordinates of the simplified system,  $\mathbf{M}$  is the inertia matrix,  $\mathbf{C}(\mathbf{q}, \dot{\mathbf{q}})$  is the generalized Coriolis matrix and  $\mathbf{u}$  is the generalized forces. Assuming small angles in  $\theta$  and  $\phi$ , the generalized forces projected in the Euler angles can be approximated as resultant force and moment applied to the CM of the robot. Following this, the forces produced by the rotation of the 12 flagella can be expressed as:

$$\mathbf{F}_G = \sum_{i=1}^{12} \mathbf{F}_i; \quad \mathbf{M}_G = \sum_{i=1}^{12} (\mathbf{M}_i + \mathbf{r}_{G,i} \times \mathbf{F}_i); \quad (16)$$

We can establish the reference frame,  $C_i$ , linked to face  $i$  by using the rotation matrix  $\mathbf{R}_{fi}$ . Then, the forces and moments generated at each face can be expressed in the frame of the rigid body as  $\mathbf{F}_i(\omega_i) = \mathbf{R}_{fi}[-a_1 \cdot |\omega_i|, 0, 0]^T$  and  $\mathbf{M}_i(\omega_i) = \mathbf{R}_{fi}[-a_2 \cdot \omega_i, 0, 0]^T$ . We establish a fixed rotation direction for each flagellum; then, the absolute module can be removed, simplifying the control law and optimizing the system's performance. We choose that the flagella in the 1, 2, 5, 6, 9, 10, faces rotate counter-clockwise, while the remaining ones rotate clockwise. This deliberate choice aims to neutralize aerodynamic torques during stable and straight maneuvers (see Figure 6B). Then, the forces and moments can be expressed as follows:

$$\mathbf{F}_i(\omega_i) = \mathbf{r}_i \cdot \omega_i; \quad \mathbf{M}_i(\omega_i) = \mathbf{p}_i \cdot \omega_i \quad (17)$$

where

$$\mathbf{r}_i(\omega_i) = \mathbf{R}_{fi}[-a_1, 0, 0]^T; \quad \forall i \quad (18)$$

$$\mathbf{p}_i(\omega_i) = \begin{cases} \mathbf{R}_{fi}[-a_2, 0, 0]^T & \forall i = 1, 2, 5, 6, 9, 10 \\ \mathbf{R}_{fi}[+a_2, 0, 0]^T & \forall i = 3, 4, 7, 8, 11, 12 \end{cases} \quad (19)$$

Expressions (17) can be simplified as follows:

$$\mathbf{M}_G = \sum_{i=1}^6 \underbrace{(\mathbf{p}_{k(i)} + \mathbf{r}_{G,k(i)} \times \mathbf{r}_{k(i)})}_{\mathbf{s}_{k(i)}} \underbrace{(\omega_{k(i)} - \omega_{k(i)+1})}_{\Omega_i}; \quad \mathbf{F}_G = \sum_{i=1}^6 \mathbf{r}_{k(i)} \underbrace{(\omega_{k(i)} - \omega_{k(i)+1})}_{\Omega_i}; \quad (20)$$

where  $k(i) = (i-1) \cdot 2 + 1$ ,  $\mathbf{r}_i = -\mathbf{r}_{i+1}$ ,  $\mathbf{p}_i = -\mathbf{p}_{i+1}$  and  $\mathbf{r}_{Gi} \times \mathbf{r}_i = -\mathbf{r}_{G,i+1} \times \mathbf{r}_{i+1}$  due to the symmetry of the system (see Figure 6A). Therefore, the resultant forces and moments applied to the CM, using the new control input  $\boldsymbol{\Omega} = [\Omega_1, \Omega_2, \dots, \Omega_6]^T$ , can be represented in matrix form as follows:

$$\mathcal{F}_G = [\mathbf{M}_G^T, \mathbf{F}_G^T]^T = \boldsymbol{\Xi}(\Theta) \cdot \boldsymbol{\Omega} \quad (21)$$

where  $\boldsymbol{\Xi}(\Theta) \in \mathbb{R}^{6 \times 6}$  is a constant matrix whose columns are  $[\mathbf{s}_{k(i)}^T, \mathbf{r}_{k(i)}^T]^T$ . Additionally, we incorporate the effects of the fluid on the body through the term  $\mathbf{F}(\mathbf{q}, \dot{\mathbf{q}})$ , which encompasses gravitational forces and fluid-body interactions including buoyancy, drag, lift, and added mass. The details of  $\mathbf{F}(\mathbf{q}, \dot{\mathbf{q}})$  for the rigid body are described in Section 2.1 for the shell of the system. Consequently, the simplified dynamic equation can be formulated as follows:

$$\mathbf{M}\ddot{\mathbf{q}} + \underbrace{\mathbf{C}(\mathbf{q}, \dot{\mathbf{q}})\dot{\mathbf{q}} - \mathbf{F}(\mathbf{q}, \dot{\mathbf{q}})}_{\boldsymbol{\zeta}(\mathbf{q}, \dot{\mathbf{q}})} = \boldsymbol{\Upsilon}(\boldsymbol{\psi}) \cdot \boldsymbol{\Xi}(\Theta) \cdot \boldsymbol{\Omega} \quad (22)$$

**Remark 1.** The rotation direction of each flagellum remains unchanged in the predefined configuration because any alteration does not impact the direction of the thrust; it only affects the moment's direction. This assumption simplifies the control law by removing the absolute value in the thrust function.

**Remark 2.** The magnitude of the angular speed, denoted by  $\omega_i$ , is inherently positive. Conversely, the new control input  $\Omega_i$  can assume any real value. To generate a positive  $\Omega_i$ ,  $\omega_i$  is actuated while keeping  $\omega_{i+1}$  zero. On the contrary, to generate a negative  $\Omega_i$ ,  $\omega_i$  is kept zero, and  $\omega_{i+1}$  is actuated.

## 4.2 Control law

In this section we will develop a control strategy for controlling the position and orientation  $\boldsymbol{\psi}$  of the system, provided that the generalized coordinates of the system associated with the main body,  $\mathbf{q}$ , and its derivatives are known. As the orientation angles  $\phi$  and  $\theta$  exhibit inherent stability by design, we abstain from direct control of these variables. This allows us to streamline the control technique, enhancing computational efficiency. Consider the nonlinear system described in (22), we can control the coordinates  $\bar{\mathbf{q}} = [\boldsymbol{\psi}, x, y, z]^T$  by taking the four last

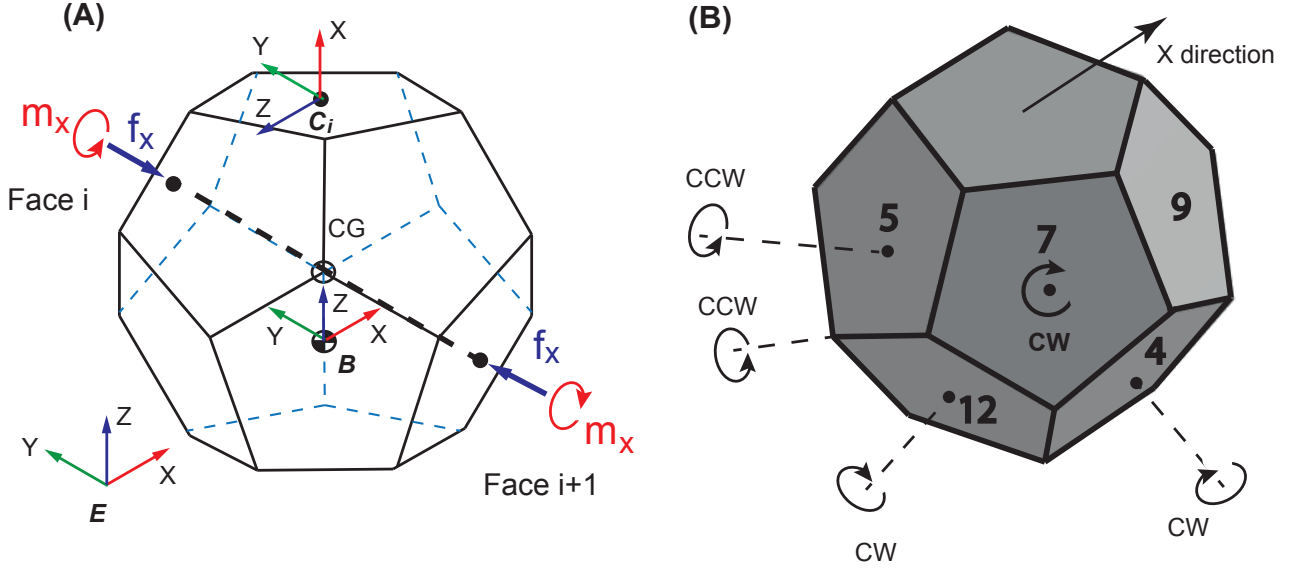

Figure 6: Zodiac main body representation: (A) Representation of the different frames and exerted forces/moments acting on the robot. (B) Indication of rotational directions for each flagellum.

equations which correspond with those coordinates as follows:

$$\Omega = (\bar{\Upsilon} \cdot \bar{\Xi}(\Theta))^\dagger \cdot (v + \bar{\zeta}(q, \dot{q})) \quad (23)$$

where we denote the pseudo-inverse of a matrix as  $(\bullet)^\dagger$ , and let  $v$  be a new input that cancels the nonlinearities, thereby transforming the system into:

$$\bar{M} \cdot \ddot{q} = v \quad (24)$$

The design of a tracking controller for this double-integrator relation can be easily obtained through a proportional-derivative (PD) controller as follows:

$$v = \bar{M}(\ddot{q}^* - K_d(\dot{q} - \dot{q}^*) - K_p(q - q^*)), \quad (25)$$

with  $K_d$  and  $K_p$  being positive constants, the tracking error of the closed loop system is exponentially stable.

Remark 1 and 2 enable the elimination of the absolute value in the thrust function, facilitating the definition of the new control input  $\Omega$ . This simplifies the control law and guarantees that the system (22) becomes differentially flat.

### 4.3 Controller implementation for experimental tests

As our experimental setup lacks a tracking system, we are unable to provide feedback on planar coordinates ( $x$  and  $y$ ) for the real prototype. To accommodate this limitation, we have made slight modifications to the control law (23)-(25) to enable the execution of various trajectories with the system. We make the assumption that the term  $\bar{\zeta}(q, \dot{q})$  is negligible due to the system's slow velocity. Moreover, we implement closed-loop control for the

depth and orientation about the vertical axis ( $\psi$ ). Meanwhile, the planar movement ( $x$  and  $y$ ) was controlled in an open-loop manner by commanding a desired acceleration  $\ddot{\mathbf{q}}^*$ . As a result, the control law can be simplified to:

$$\mathbf{\Omega} = (\overline{\mathbf{r}} \cdot \overline{\mathbf{\Xi}}(\Theta))^{\dagger} \cdot \overline{\mathbf{M}} \cdot \begin{pmatrix} \ddot{\psi}^* - K_d(\dot{\psi} - \dot{\psi}^*) - K_p(\psi - \psi^*) \\ \ddot{x}^* \\ \ddot{y}^* \\ \ddot{z}^* - K_d(\dot{z} - \dot{z}^*) - K_p(z - z^*) \end{pmatrix}; \quad (26)$$

## References

- [1] Armanini C, Farman M, Calisti M, Giorgio-Serchi F, Stefanini C, Renda F. Flagellate Underwater Robotics at Macroscale: Design, Modeling, and Characterization. *IEEE Transactions on Robotics*. 2022;38(2):731-47.
- [2] Mathew AT, Hmida IMB, Armanini C, Boyer F, Renda F. SoRoSim: A MATLAB Toolbox for Hybrid Rigid-Soft Robots Based on the Geometric Variable-Strain Approach. *IEEE Robotics and Automation Magazine*. 2022.
- [3] Ben Hmida I, Feliu-Talegon D, Mathew AT. ZodiAq digital twin in SoRoSim: ZodiAq Branch; 2023. GitHub repository, ZodiAq branch. Available from: <https://github.com/Ikhlaz-Ben-Hmida/SoRoSim/tree/ZodiAq>.
- [4] Samir B. Design and control of quadrotors with application to autonomous flying. Project report, Ecole Polytechnic. 2007.
